# Supplementary material for: Representation Learning for Weakly Supervised Relation Extraction
Source: arXiv:2105.00815 source file (2024-03-16)
Supplement: Supplementary file 1 [file appendix.tex]

% \appendix
\newpage
\appendix
\chapter{Appendix A}
\section{Results of Experiments} \label{App:AppendixA}
\begin{table*}
  \centering
  \begin{adjustbox}{width=1\textwidth, height=0.5\textheight}
  \input table/ret1.tex
  \end{adjustbox}
  \caption{Performance of $B-H$}
\end{table*}
\begin{table*}
  \centering
  \begin{adjustbox}{width=1\textwidth, height=0.5\textheight}
  \input table/ret2.tex
  \end{adjustbox}
  \caption{Performance of $B-HL$}
\end{table*}
\begin{table*}
  \centering
  \begin{adjustbox}{width=1\textwidth, height=0.5\textheight}
  \input table/ret3.tex
  \end{adjustbox}
  \caption{Performance of $M-E-L$}
\end{table*}
\begin{table*}
  \centering
  \begin{adjustbox}{width=1\textwidth, height=0.5\textheight}
  \input table/ret4.tex
  \end{adjustbox}
  \caption{Performance of $M-E-LUE$}
\end{table*}
\begin{table*}
  \centering
  \begin{adjustbox}{width=1\textwidth, height=0.5\textheight}
  \input table/ret5.tex
  \end{adjustbox}
  \caption{Performance of $M-E-LUEW$}
\end{table*}
\begin{table*}
  \centering
  \begin{adjustbox}{width=1\textwidth, height=0.5\textheight}
  \input table/ret6.tex
  \end{adjustbox}
  \caption{Performance of $M-EW-L$}
\end{table*}
\begin{table*}
  \centering
  \begin{adjustbox}{width=1\textwidth, height=0.5\textheight}
  \input table/ret7.tex
  \end{adjustbox}
  \caption{Performance of $M-EW-LUE$}
\end{table*}
\begin{table*}
  \centering
  \begin{adjustbox}{width=1\textwidth, height=0.5\textheight}
  \input table/ret8.tex
  \end{adjustbox}
  \caption{Performance of $M-EW-LUEW$}
\end{table*}
